# Supplementary material for: Correlated electron behavior of metalorganic molecules: insights from density functional theory combined with many-body effects using exact diagonalization
Source: arXiv:1506.07973 source file (2015-06-26)
Supplement: Supplementary file 1 [file SI_Bhandary1.pdf]

# Supplementary Information: Correlated electron behavior of metalorganic molecules: insights from density functional theory combined with many-body effects using exact diagonalization

Sumanta Bhandary,[1,*] Malte Schüler,[2] Patrik Thunström,[3] Igor di Marco,[1] Barbara Brena,[1] Olle Eriksson,[1] Tim Wehling,[2] and Biplab Sanyal[1,†]

[1]*Department of Physics and Astronomy, Uppsala University, Box 516, 751 20 Uppsala, Sweden*
[2]*Institute for Theoretical Physics, University of Bremen, Otto-Hahn-Allee 1, 28359 Bremen, Germany and Bremen Center for Computational Materials Science, University of Bremen, Am Falturm 1, 28359, Bremen, Germany*
[3]*Institute of Solid State Physics, Vienna University of Technology, Wiedner Hauptstrasse 8 -10, 1040 Wien, Austria*

In this Supplementary information, we show the hybridization functions for (i) stretched FeP and (ii) FePc molecules. Also, a model Hamiltonian approach has been considered to analyze the behavior of static crystal field as a function of hybridization between Fe-d and N-p orbitals in FeP.

In Fig. 1 of the Supplementary Information, we show the calculated hybridization functions for FeP with Fe-N bond length, 2.11 Å, which is enhanced compared to that of the ground state. This change in bond length is reflected in the difference in hybridization strengths and static crystal fields for stretched and unstretched (shown in the main paper) FeP. The stretching of Fe-N bond weakens the hybridization and hence, the coupling strength V as well as the static crystal field. A quantitative description of this change can be observed in Fig. 2 in the main paper.

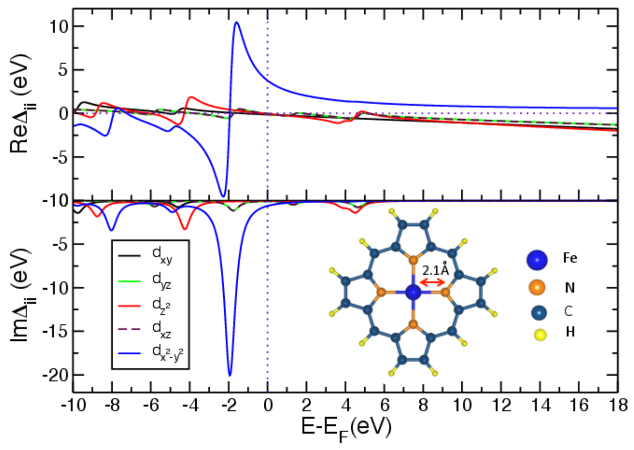


FIG. 1. (Color online) Real and imaginary parts of the hybridization function for Fe in FeP with enhanced Fe-N bond lengths (2.11 Å), calculated with PBE in the non spin-polarized mode. FeP is shown in the inset with the atoms labeled by their types.

In Fig. 2, the calculated hybridization function for iron phthalocyanine (FePc) is shown along with the geometry of the molecule. FePc has four extra nitrogen atoms connecting four C -rings resulting in a slightly shorter Fe-N bond length of 1.94 Å. Hence, the parameters extracted from the calculated hybridization function are different from FeP. Specifically, the real part of the hybridization function of $d_{x^2-y^2}$ orbital has a much bigger intensity than that of FeP. This increases the strength of hybridization for FePc (3.16 eV for FeP and 3.39 eV for FePc) and hence, it is difficult to switch the spin state of Fe in FePc compared to FeP. The difference in bath energies in FeP and FePc can be attributed to the structural differences between the two molecules.

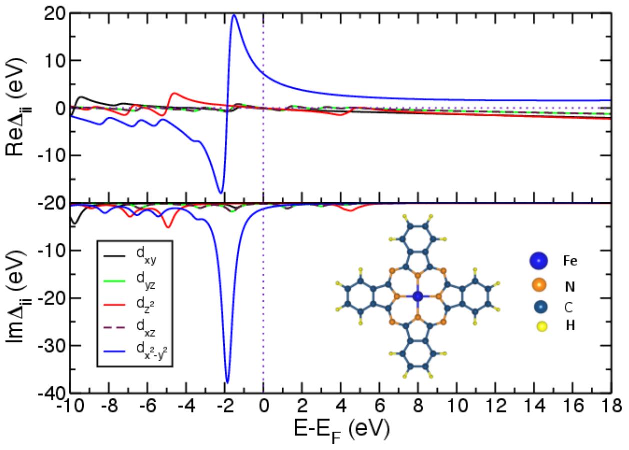


FIG. 2. (Color online) Real and imaginary parts of the hybridization function for Fe in FePc calculated with PBE in the non spin-polarized mode. FePc is shown in the inset with the atoms labeled by their types.

The spin phase diagram in Fig. 2 in the main text depicts spin phases, defined by the strength of crystal field ($V_{cryst}$) exerted on the central Fe atom and its hybridization (V) with the neighboring atoms. We can identify characteristic energy contribution for specific spin phases, categorized in four terms as follows:

- V $\rightarrow$ 0 defines an atomic situation and with V$_{cryst}$ $\geq$ V$_{transition}$ (as in Fig. 2 in the main text) an intermediate spin state (S=1) is achieved. Six electrons in $Fe^{2+}$ are distributed in d$_{rest}$ (the remaining degenerate Fe orbitals excluding d$_{x^2-y^2}$). The major energy gain is of crystal field energy, defined as E$_{LS}$=V$_c$(1-n$_{x^2-y^2}$+(2-n$_p$)) and spin phase dominated by this energy gain is termed as atomic **'low spin'** state (expressed in red color). V$_c$(1-n$_{x^2-y^2}$) provides the energy gain for not having an electron on d$_{x^2-y^2}$. Moreover we have one bath orbital containing 2 electrons. For finite V, the electron transfer from the bath to impurity (in d$_{x^2-y^2}$ orbital) is taken in to account by (2-n$_p$). Subtraction of this number from n$_{x^2-y^2}$ provides explicitly the energy gain for not having an impurity electron in d$_{x^2-y^2}$ orbital.

- With V$\rightarrow$ 0, as we reduce V$_{cryst}$ $\leq$ V$_{transition}$, it is more favourable to gain energy by exchange interaction, which favors maximization of spin, even at the cost of crystal field energy. The phase is termed as atomic **'high spin'** phase, expressed in blue and is characterized by an energy gain of exchange origin, E$_{HS}$=I$_{ex}$S$^{d_{x^2-y^2}}$ $\cdot$ $S^{rest}$. Where I$_{ex}$ is Stoner parameter and S$^{d_{x^2-y^2}}$ and S$^{rest}$ are spins in d$_{x^2-y^2}$ and d$_{rest}$, respectively.

- With a significantly large V, the major contribution in energy gain comes from hopping and as long as V$_{cryst}$ $\geq$ V$_{transition}$, the electrons in d$_{x^2-y^2}$ come from the bath via bonding orbital. This occupation is non spin-polarized and does not contribute to the exchange energy gain. The spin state remains S=1 but is governed by bonding rather than crystal field only. The characteristic energy term : E$_{BS}$= V(d$^\dagger$ p + h.c.)+E$_p$(n$_p$-2)+(E$_d$-V$_c$)(2-n$_p$), where the first term is hopping and the second and third terms are energy costs of losing electron from p-orbital and adding to d$_{x^2-y^2}$ orbitals, respectively. The spin phase is termed as **'bonding state'** low spin phase and is depicted by green color.

- As V$_{cryst}$ is reduced for large V, an electron from d$_{rest}$ jumps to anti-bonding orbital containing predominantly d$_{x^2-y^2}$ in order to gain in exchange energy but at a cost of crystal field energy. The phase is termed as **'anti-bonding state'** high spin phase, which differs from atomic high spin state as the molecular anti-bonding orbital is comprised of both Fe-d$_{x^2-y^2}$ and N-p orbitals. The presence of an electron in d$_{x^2-y^2}$ orbital reduce electron hopping from N-p significantly. Moreover, there is also an electron transfer from d$_{x^2-y^2}$ to N-p via anti-bonding orbital. The effect can be seen at the right corner of Fig. 2 in the main text, where the blue region is suppressed partially by green.

The phase boundary, on the other hand establishes a relation between V and V$_{cryst}$, which is explicitly seen from our ED calculation of spin crossover. Fig. 2 in the main text exhibits a parabolic behavior of V-V$_{cryst}$ relation at the spin-crossover point. This particular curving of the phase boundary can be explained with the following one particle model.

The subblock of the single particle terms in Hamiltonian involving the dx-y orbitals and their hybridization the N-p ligands reads,

$$H = (E_d + V_{cryst})d^\dagger d + E_p p^\dagger p + (V d^\dagger p + h.c.) \quad (1)$$

where $E_d$ and $E_p$ are the onsite energies of Fe-d and N-p orbitals respectively. Note that crystal field is only applied to d$_{x^2-y^2}$ orbital and hopping of electron is also allowed to(from) d$_{x^2-y^2}$ orbital from (to) N-p orbitals. This approximation is done in accordance with our observation in the hybridization function, discussed in the main text.

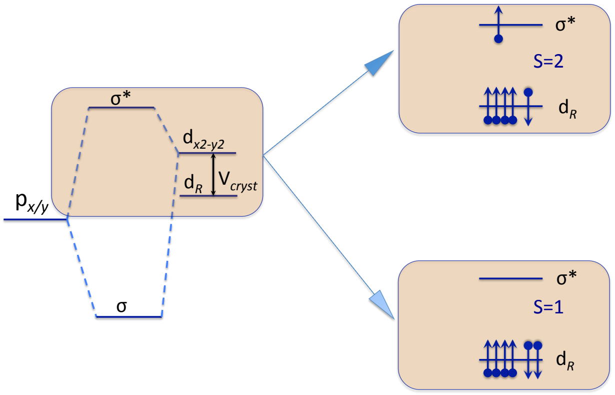


FIG. 3. (Color online) The schematic picture describing the d-p model. On the left, the bonding $\sigma$ and antibonding $\sigma^\star$ orbitals due to the hybridization between Fe-d and N-p orbitals are shown. On the right, the two possible scenario of high and low spin states are illustrated.

Solving this Hamiltonian one can arrive to expressions of bonding (E$_b$) and antibonding levels (E$_a$), given as

$$E_{a/b} = (\bar{E} + \frac{V_{cryst}}{2}) \pm \sqrt{(\Delta E + \frac{V_{cryst}}{2})^2 + V^2} \quad (2)$$

where, $\bar{E} = (E_d + E_p)/2$ and $\Delta E = (E_d - E_p)/2$

Now, with the reference level, i.e., the five-fold degenerate $d$ level before subjected to crystal field, $d_R = E_d$, the high (HS) and low spin (LS) state energies can be defined on a mean filed level [1],

$$E_{HS} = E_a - Im^2/4 = E_a - 4I \quad (3)$$

$$E_{LS} = E_d - Im^2/4 = E_d - I \quad (4)$$

$I$ is the local exchange integral and $m$ is the magnetic moment, which is m=S=2 in the HS and m=S=1 in the LS state. At the crossover point, $E_{HS} = E_{LS}$, which yields,

$$V_{cryst} = A - BV^2 \tag{5}$$

where $A = 3I$, and $B = 1/(3I + E_d - E_p)$.

The above parabolic relationship between $V_{cryst}$ and $V^2$ (Eqn. 5) at the phase boundary between HS and LS states is obtained from simplified considerations of our analytic calculations. It should be noted that this behavior is also observed in our explicit calculations by varying $V_{cryst}$ and V in the Anderson impurity model, presented in the main text. It is also interesting to note that the parameters $A$ and $B$ in the quadratic equation are related to physical quantities like local exchange integral and p/d energy level position.

* Present address: Institute of Solid State Physics, Vienna University of Technology, Wiedner Hauptstrasse 8 -10, 1040 Wien, Austria

† Biplab.Sanyal@physics.uu.se

[1] M. S. S. Brooks and B. Johansson, J. Phys. F: Met. Phys. **13** L197-L202 (1983)
